# Supplementary material for: SemDiff: Binary Similarity Detection by Diffing Key-Semantics Graphs
Source: arXiv:2308.01463 source file (2026-10-27)
Supplement: Supplementary file 1 [file appendix.tex]

\begin{table*}[ht]
\footnotesize
%\begin{tabular}{p{1.4cm}p{0.7cm}p{0.7cm}p{0.7cm}p{0.7cm}p{0.7cm}p{0.7cm}}
\begin{tabular}{c| c | c | c | c | c | c }
 \hline
\multirow{2}{*}{Program} & BinDiff & funcsimsrch & Asm2Vec & Gemini & Palmtree& \name  \\%& \multicolumn{6}{c}{($O3$ vs. $O1$, $Os$ vs. $O1$} \\
  &O3-O1 OS-O1&O3-O1 OS-O1&O3-O1 OS-O1&O3-O1 OS-O1&O3-O1 OS-O1&O3-O1 OS-O1\\\hline
 openssl &(0.620,0.519) & (0.126,0.123) & (0.880,0.923) & (0.463,0.402) & (0.675,0.612) & (\textbf{0.883},\textbf{0.926})\\ 
 %\hline
 libtomcrypt & (0.394,0.151) & (0.127,0.098) & (0.897,\textbf{0.923}) & (0.208,0.153) & (0.335,0.309) &(\textbf{0.901},0.792) \\
 %\hline
 coreutils & (0.254,0.431)  &(0.096,0.117)  & (0.790,\textbf{0.887}) & (0.303,0.295) & (0.506,0.502) &(\textbf{0.799},0.849)\\
 %\hline
 libMagickCore & (0.235,0.203)  &(0.061,0.059)  &(\textbf{0.909},\textbf{0.905}) & (0.394,0.231) & (0.542,0.390) & (0.845,0.802)\\
 %\hline
 libMagickWand & (0.192,0.162)  & (0.041,0.039)  & (0.925,0.862) & (0.192,0.152) & (0.265,0.236) &(\textbf{0.960},\textbf{0.920})\\ 
 %\hline
 libgmp & (0.392,0.480)  & (0.239,0.257)  & (0.790,0.847) & (0.431,0.401) & (0.631,0.612) &(\textbf{0.861},\textbf{0.857})\\ 
 %\hline
 curl & (0.566,0.700)  &(0.263,0.230)  & (0.818,0.900) & (0.571,0.510) & (0.813,0.888) &(\textbf{0.869},\textbf{0.950})\\ 
 %\hline
 sqlite3 & (0.151,0.639)  & (0.128,0.196)  & (0.670,0.925) & (0.179,0.301) &(0.359,0.600) &(\textbf{0.740},\textbf{0.931})\\ 
 %\hline
 libz & (0.191,0.511)  & (0.236,0.295) & (\textbf{0.775},0.955) & (0.306,0.402) & (0.424,0.680) &(0.730,\textbf{1.000})\\ 
 %\hline
 plink & (0.310,0.565)  & (0.110,0.148)  & (0.693,0.893) & (0.369,0.408) & (0.591,0.628) &(\textbf{0.732},\textbf{0.936})\\ 
 %\hline
 pscp & (0.310,0.596) & (0.095,0.120)  & (0.680,0.896) & (0.347,0.418) &(0.549,0.635) &(\textbf{0.706},\textbf{0.937})\\ 
 %\hline
 psftp & (0.323,0.603)  & (0.101,0.124)  & (0.676,0.889) & (0.355,0.426) & (0.547,0.644) &(\textbf{0.716},\textbf{0.930})\\ 
 %\hline
 puttygen & (0.319,0.584) & (0.059,0.066)  & (0.586,0.843) &(0.324,0.414) & (0.502,0.589) &(\textbf{0.652},\textbf{0.920})\\ 
 \hline
 Avg. &(0.327,0.473)  & (0.129,0.144) & (0.776,0.896)  & (0.342,0.347) & (0.518,0.563) & (\textbf{0.800},\textbf{0.904})\\ 
 \hline

\end{tabular}
\caption{Libraries compiled by GCC5.4.0 with different optimization levels. funcsimsrch is short for functionsimsearch.}
\label{tab:gcc_appendix}
\end{table*}

\begin{table*}[h]
\footnotesize
\begin{tabular}{c| c | c | c | c | c | c }
%{p{1.4cm}p{0.7cm}p{0.7cm}p{0.7cm}p{0.7cm}p{0.7cm}p{0.7cm}}
 \hline
\multirow{2}{*}{Program} & BinDiff & funcsimsrch & Asm2Vec &Gemini & Palmtree & \name  \\%& \multicolumn{6}{c}{(CLANG $O1$ vs. GCC $O0$, CLANG $O3$ vs. GCC $O1$, CLANG $O3$ vs. GCC $O0$)} \\
  &O1-O0 O3-O1 O3-O0&O1-O0 O3-O1 O3-O0&O1-O0 O3-O1 O3-O0&O1-O0 O3-O1 O3-O0&O1-O0 O3-O1 O3-O0&O1-O0 O3-O1 O3-O0 \\
 \hline
 openssl & (0.254, 0.226,0.116)  & (0.042, 0.049, 0.047)  & (0.763, 0.844, 0.723) & (0.179, 0.224, 0.175) & (0.096, 0.224, 0.131) & (\textbf{0.780}, \textbf{0.878}, \textbf{0.733})\\ 
 %\hline
 libtomcrypt & (0.043, 0.134, 0.055)  & (0.028, 0.043, 0.033)  &(0.651, \textbf{0.853}, 0.614) & (0.029, 0.060, 0.027) & (0.030, 0.060, 0.04) & (\textbf{0.751}, 0.799, \textbf{0.72})\\ 
 %\hline
 coreutils & (0.256, 0.106, 0.027)  & (0.056, 0.073, 0.031)  & (0.554, 0.780, 0.426) & (0.102, 0.146, 0.076) & (0.166, 0.241, 0.135) &(\textbf{0.650}, \textbf{0.810}, \textbf{0.529}) \\ 
 %\hline
 libMagickCore & (0.133, 0.142, 0.071)  & (0.047, 0.036, 0.027)  & (0.610, \textbf{0.861}, 0.599) & (0.095, 0.148, 0.084) & (0.146, 0.200, 0.09) & (\textbf{0.792}, 0.823, \textbf{0.728})\\ 
 %\hline
 libMagickWand & (0.085, 0.098, 0.042)  & (0.038, 0.032, 0.023)  & (0.360, 0.760, 0.339) & (0.056, 0.120, 0.048) & (0.054, 0.060, 0.054) & (\textbf{0.901}, \textbf{0.929}, \textbf{0.875})\\ 
 %\hline
 libgmp & (0.222, 0.280, 0.292)  & (0.156, 0.174, 0.14)  & (\textbf{0.697}, 0.581, \textbf{0.776}) & (0.163, 0.219, 0.218) & (0.215, 0.253, 0.243) & (0.610, \textbf{0.683}, 0.649)\\ 
 %\hline
 curl & (0.348, 0.245, 0.259)  & (0.087, 0.255, 0.062)  & (0.761, 0.872, \textbf{0.802}) & (0.222, 0.310, 0.198) & (0.231, 0.380, 0.231) & (\textbf{0.848}, \textbf{0.904}, 0.79)\\ 
 %\hline
 sqlite3 & (0.318, 0.052, 0.017)  & (0.127, 0.070, 0.056)  & (0.651, 0.503, 0.419) & (0.085, 0.059, 0.03) & (0.090, 0.088, 0.045) & (\textbf{0.752}, \textbf{0.643}, \textbf{0.469}) \\ 
 %\hline
 libz & (0.690, 0.057, 0.025) & (0.287, 0.230, 0.198)  & (0.793, 0.724, 0.642) & (0.190, 0.280, 0.171) & (0.270, 0.305, 0.195) & (\textbf{0.816}, \textbf{0.793}, \textbf{0.704})\\ 
 %\hline
 plink & (0.276, 0.249, 0.05)  & (0.084, 0.098, 0.053)  & (0.644, 0.659, 0.433) & (0.137, 0.200, 0.14) & (0.134, 0.252, 0.13) & (\textbf{0.763}, \textbf{0.763}, \textbf{0.567})\\ 
 %\hline
 pscp & (0.254, 0.226, 0.045)  & (0.074, 0.081, 0.049)  & (0.647, 0.689, 0.43) & (0.140, 0.195, 0.139) & (0.128, 0.230, 0.125) & (\textbf{0.778}, \textbf{0.746}, \textbf{0.558})\\ 
 %\hline
 psftp & (0.294, 0.212, 0.055)  & (0.078, 0.080, 0.053)  & (0.644, 0.672, 0.417) & (0.148, 0.196, 0.139) & (0.112, 0.218, 0.123) & (\textbf{0.775}, \textbf{0.753}, \textbf{0.545})\\ 
 %\hline
 puttygen & (0.399, 0.282, 0.135)  & (0.042, 0.067, 0.026)  & (0.568, 0.566, 0.334) & (0.156, 0.162, 0.151) & (0.143, 0.212, 0.122) & (\textbf{0.722}, \textbf{0.695}, \textbf{0.495})\\ 
 \hline
 Avg. & (0.275, 0.178, 0.089)  & (0.088, 0.099, 0.060)  & (0.642, 0.720, 0.548) & (0.131, 0.178, 0.123) & (0.140, 0.210, 0.128) & (\textbf{0.764}, \textbf{0.786}, \textbf{0.635})\\ 
 \hline
\end{tabular}
\caption{Binary comparison result when using different compilers and optimization levels. (funcsimsrch is short for functionsimsearch}
\label{tab:clang}
\end{table*}

\begin{table*}[h]
\centering
\footnotesize
\begin{tabular}{p{0.5cm}cp{0.5cm}p{0.5cm}p{0.5cm}p{0.5cm}p{0.5cm}p{0.5cm}}
 \hline
  Program & Version & \rotatebox[origin=c]{270}{BinDiff} & \rotatebox[origin=c]{270}{funcsimsrch} & \rotatebox[origin=c]{270}{Asm2Vec} & \rotatebox[origin=c]{270}{Gemini} & \rotatebox[origin=c]{270}{Palmtree} & \rotatebox[origin=c]{270}{\name}  \\ 
  \hline
 
 %\hline
  libtomcrpt &  \multicolumn{1}{r}{1.18.0 vs. 1.18.2} & 0.776 &0.276 &0.736 & 0.434 &0.446&\textbf{0.863}\\ 
 %\hline
  & \multicolumn{1}{r}{1.18.1 vs. 1.18.2}& 0.785 &0.275 &0.750 &0.418 &0.467 &\textbf{0.869} \\ 
  & \multicolumn{1}{r}{1.18.0rc3 vs 1.18.2}& 0.783 &0.28 &0.739 &0.409 &0.469 &\textbf{0.856} \\ 
 \hline

 \hline

 \multirow{3}{*}{libgmp} & \multicolumn{1}{r}{6.1.0 vs. 6.2.1}&  0.287 &0.150 &\textbf{0.523} &0.203 &0.251 &0.477
\\ 
 %\hline
   &  \multicolumn{1}{r}{6.1.2 vs. 6.2.1} & 0.280 &0.148 &\textbf{0.511} &0.213 &0.257 &0.478
\\ 
 %\hline
  & \multicolumn{1}{r}{6.2.0 vs. 6.2.1}& 0.333 &0.180 &\textbf{0.550}  &0.261 &0.285 &0.527
 \\ 
 \hline
 Avg.&&0.300 &0.159 &\textbf{0.528}  &0.226 &0.264 &0.494 \\ 
 \hline
 \multirow{3}{*}{libmgkc} & \multicolumn{1}{r}{7.1.0-8 vs. 7.1.0-10}  & 0.845 & 0.248 &0.738 &0.524 &0.527 &\textbf{0.869}
\\ 
 %\hline
   &  \multicolumn{1}{r}{7.1.0-9 vs. 7.1.0-10} & 0.846 & 0.254 & 0.737 &0.869 &0.520 &0.532
 \\ 
 %\hline
  & \multicolumn{1}{r}{7.1.0-11 vs. 7.1.0-10}& 0.832 &0.244 &0.739  &0.539 &0.538 &\textbf{0.859}
 \\ 
 \hline
 
 \multirow{3}{*}{libmgkw} & \multicolumn{1}{r}{7.1.0-8 vs. 7.1.0-10} & 0.968 &0.073 &0.538 &0.146 &0.181 &\textbf{0.986}
 \\ 
 %\hline
   &  \multicolumn{1}{r}{7.1.0-9 vs. 7.1.0-10} &0.968 &0.074 &0.540 &0.148 &0.186 &\textbf{0.989}
 \\ 
 %\hline
  & \multicolumn{1}{r}{7.1.0-11 vs. 7.1.0-10}& 0.968 &0.074 &0.534 &0.139 &0.168 &\textbf{0.988}
 \\ 
 \hline

 \multirow{3}{*}{sqlite3} & \multicolumn{1}{r}{3.35.5 vs. 3.37.0} & \textbf{0.991} &0.405 &0.928 &0.526 &0.730 &0.985
 \\ 
 %\hline
   &  \multicolumn{1}{r}{3.36.5 vs. 3.37.0} & \textbf{0.994} &0.411 &0.942 &0.528 &0.721 &0.987
\\ 
 %\hline
  & \multicolumn{1}{r}{3.37.1 vs. 3.37.0}& \textbf{1.0} &0.431 &0.940 &0.548 &0.734 &0.991
 \\ 
 \hline

 \multirow{3}{*}{plink} & \multicolumn{1}{r}{0.71 vs. 0.74} & 0.972 &0.231 &0.847 &0.484 &0.618 &\textbf{0.977}
  \\ 
 %\hline
   &  \multicolumn{1}{r}{0.72 vs. 0.74} & 0.974 &0.232 &0.851 &0.493 &0.637 &\textbf{0.986}
\\ 
 %\hline
  & \multicolumn{1}{r}{0.73 vs. 0.74}& 0.973 &0.240 &0.858 &0.482 &0.635 &\textbf{0.987}
 \\ 
 \hline
 
 \multirow{3}{*}{pscp} & \multicolumn{1}{r}{0.71 vs. 0.74} & 0.975 &0.217 &0.864 &0.489 &0.668 &\textbf{0.977}
 \\ 
 %\hline
   &  \multicolumn{1}{r}{0.72 vs. 0.74} &0.975 &0.223 &0.872  &0.478 &0.646 &\textbf{0.986}
 \\ 
 %\hline
  & \multicolumn{1}{r}{0.73 vs. 0.74}& 0.975 &0.232 &0.878 &0.483 &0.639 &\textbf{0.983}
 \\ 
 
 \hline
 \multirow{3}{*}{psftp} & \multicolumn{1}{r}{0.71 vs. 0.74} &0.968 &0.230 &0.871 &0.495 &0.636 &\textbf{0.982}
 \\ 
 %\hline
   &  \multicolumn{1}{r}{0.72 vs. 0.74} & 0.975 &0.229 &0.889 &0.476 &0.654 &\textbf{0.985}
\\ 
 %\hline
  & \multicolumn{1}{r}{0.73 vs. 0.74}& 0.975 &0.228 &0.880  &0.497 &0.633 &\textbf{0.985}
 \\ 
 \hline
 
 \multirow{3}{*}{puttygen} & \multicolumn{1}{r}{0.71 vs. 0.74} & 0.946 &0.174 &0.866 &0.522 &0.666 &\textbf{0.956}
 \\ 
 %\hline
   &  \multicolumn{1}{r}{0.72 vs. 0.74} & \textbf{0.963} &0.185 &0.872 &0.489 &0.670 &0.960
 \\ 
 %\hline
  & \multicolumn{1}{r}{0.73 vs. 0.74}& \textbf{0.963} &0.197 &0.849 &0.510 &0.690 &0.960
 \\ 
 \hline
 
\end{tabular}
\caption{The similarity scores are computed by 6 tools for open-source programs of different versions compiled by GCC 5.4.0. (funcsimsrch is short for functionsimsearch. Libmgkc shorts for LibMagickCore, libmgkw shorts for LibMagickWand.)}
\label{tab:cross_version_extra}
\end{table*}
